# Supplementary material for: Optimizing defect states in $(Bi_{0.3}Sb_{0.7})_{2}Te_{3}$ ternary topological insulators using indium doping
Source: arXiv:2410.06291 ancillary file (2025-08-11)
Supplement: Supplementary file 1 [file supplementary.pdf]

# Optimizing defect states in $(Bi_{0.3}Sb_{0.7})_2Te_3$ ternary topological insulators using indium doping

Kanav Sharma,[1] Ritam Banerjee,[1] Anuvab Nandi,[1] Radha Krishna Gopal,[2] and Chiranjib Mitra[1]

[1]*Department of Physical Sciences, Indian Institute of Science Education and Research Kolkata, Nadia, 741246, West Bengal, India*

[2]*Department of Physics and Material Sciences and Engineering, Jaypee Institute of Information Technology, Sector 62, Noida, India*

## I. XRD of BST and IBST

During the deposition of thin films, one or two additional BST and IBST films were prepared for each sample to facilitate characterization using techniques such as XRD, SEM, EDS, and Raman spectroscopy. Fig. 1 shows peaks associated with the chalcogen-ordered structure of these alloys (at 003, 006, 009, 0015, 0018, and 0021) for both samples, confirming the films' crystallinity. The peak intensity is lower for the IBST sample, as indicated in Fig. 1 (blue) but higher for pritine BST Fig. 1 (red).

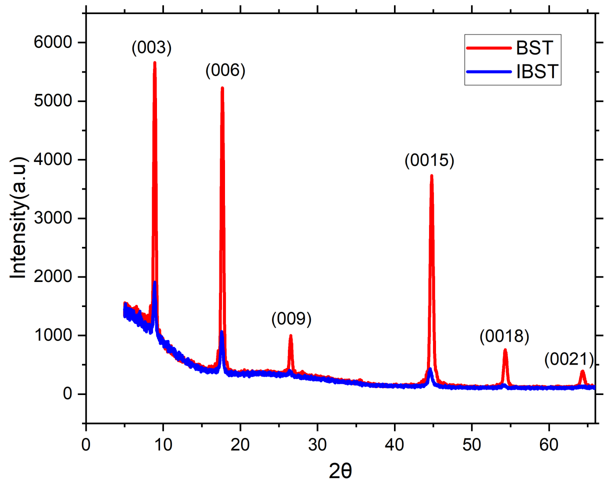


FIG. 1: XRD of BST and IBST films are shown, BST is in red and IBST in blue.

## II. Energy Dispersive X-Ray Spectroscopy(EDS)

| Elements | Weight% | Atomic% |
|---|---|---|
| Sb | 27.55 | 31.04 |
| Te | 51.11 | 54.95 |
| Bi | 21.35 | 14.01 |

TABLE I: Elemental composition of BST

| Elements | Weight% | Atomic% |
|---|---|---|
| In | 5.66 | 6.71 |
| Sb | 27.45 | 30.72 |
| Te | 45.55 | 48.64 |
| Bi | 21.35 | 13.92 |

TABLE II: Elemental composition of IBST

## III. Scanning Electron Microscopy(SEM)

SEM images reveal important details about the morphology, structure, and composition of materials at micro- to nanoscale levels. The SEM images of BST and IBST samples, shown in Fig. 2 and Fig. 3 at various magnifications, demonstrate these properties.

## IV. Temperature stability

Temperature fluctuations can introduce external disturbances to the noise signal. Noise data was collected when these fluctuations were kept below 5 mK. Fig. 4 illustrates the temperature stability with time at 250 K and 100 K, respectively.

## V. Raman spectra

The Raman spectra for these thin films are shown in Fig. 5. Both BST and IBST samples are Raman active and exhibit Raman peaks. Analysis of the spectra reveals that all the films display excellent crystallinity, with distinct Raman peaks at $107.695 cm^{-1}$ and $159.85 cm^{-1}$ for the BST sample, corresponding to the $E_g^2$ and $A_{1g}^2$ modes, respectively. The IBST sample also shows distinct Raman peaks at $107.695 cm^{-1}$ and $157.855 cm^{-1}$, corresponding to the $E_g^2$ and $A_{1g}^2$ modes, respectively.

## VI. Geometrical Structure:

Fig. 6a depicts the geometric layout of the contact pads on the films. Fig. 6b displays four contact pads, with current applied through the outer pads and voltage measured across the inner pads. The sample's channel width is 350 micrometers, and the distance between the two voltage probes is 1 mm.

## VII. Thin Film Growth:

Thin films of $(Bi_{0.3}Sb_{0.7})_2Te_3$ (S1) and indium-doped $In_{0.14}(Bi_{0.3}Sb_{0.7})_{1.86}Te_3$ (S2) were grown using Using the Pulsed Laser Deposition (PLD) technique on silicon substrates. The laser used

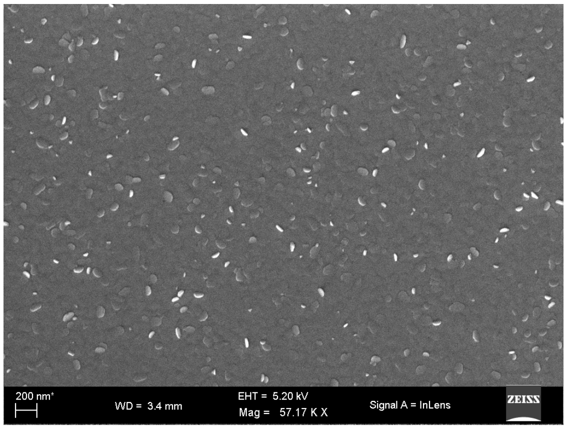


(a) SEM image at high magnification (33.29KX)

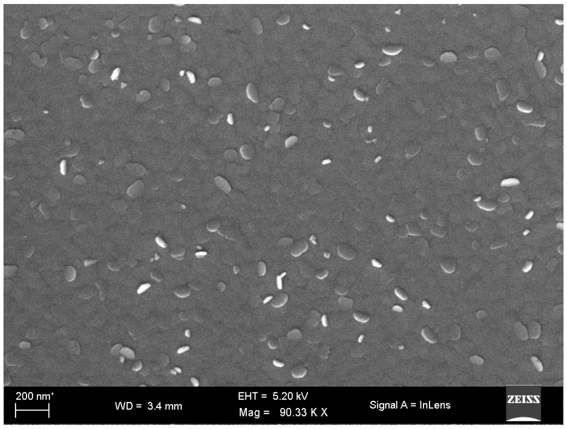


(b) Grain size with EHT voltage at 5.21KV second image.

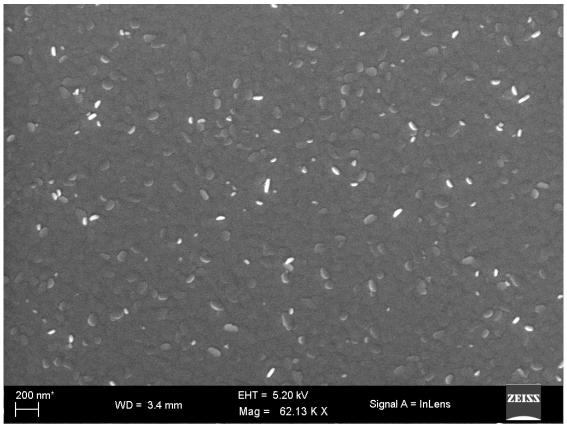


(c) Grain size with EHT voltage at 5.21KV

FIG. 2: SEM image of BST

for this purpose is a KrF-excimer with a wavelength of 248nm. We ablated individual targets of stoichiometric $(Bi_{0.3}Sb_{0.7})_2Te_3$(BST) and $In_{0.14}(Bi_{0.3}Sb_{0.7})_{1.86}Te_3$(IBST)[1, 2]. The substrates underwent a thorough cleaning process, including sequential ultrasonication with acetone and deionised water, each for 15 minutes. Thin films were grown at a temperature of 220°C with a repetition rate of 1 Hz. The energy density of the laser pulses are approximately 2.2 J/cm$^2$. The deposition was performed in the presence of argon at a partial pressure of $5 \times 10^{-1}$ mbar, having obtained a base pressure of $5 \times 10^{-6}$mbar. The film thickness was adjusted by varying the distance between the target and the substrate holder within the PLD chamber.

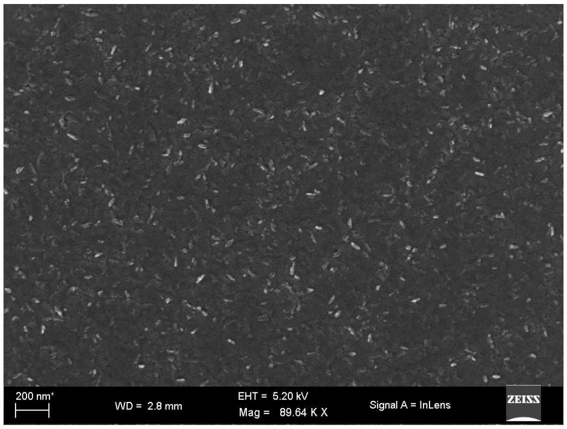


(a) SEM image at high magnification (33.29KX)

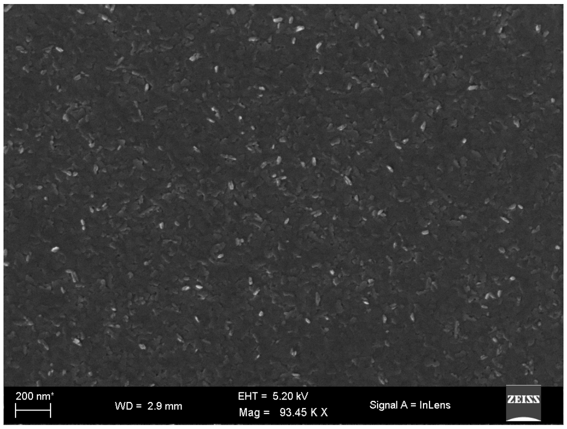


(b) Grain size with EHT voltage at 5.21KV second image.

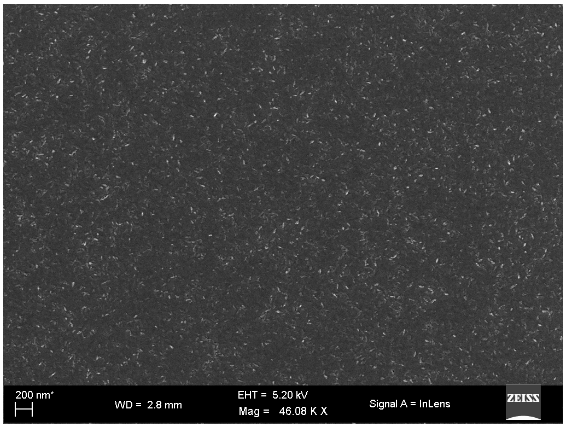


(c) Grain size with EHT voltage at 5.21KV

FIG. 3: SEM image of IBST sample

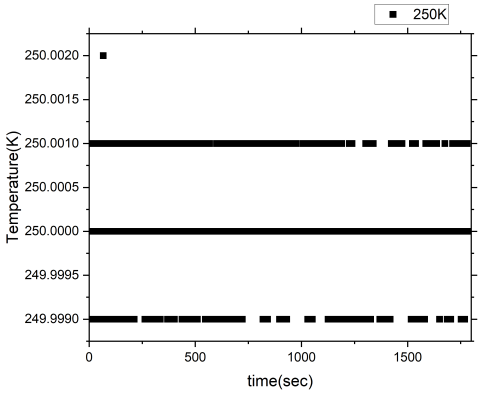


(a) Temperature fluctuations at 250K with time.

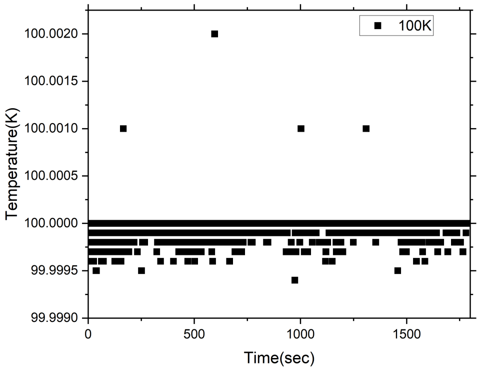


(b) Temperature fluctuations at 100K with time.

FIG. 4: Shows the fluctuations in temperature are less than 5 mK.

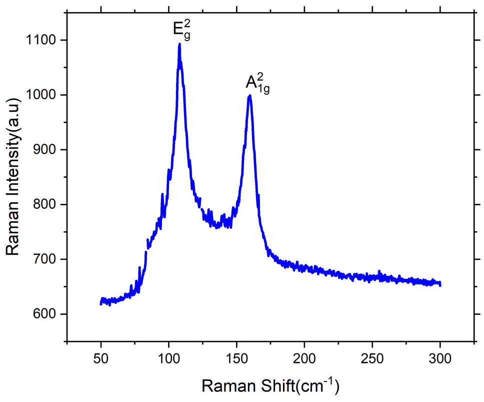


(a) Raman shift for BST sample.

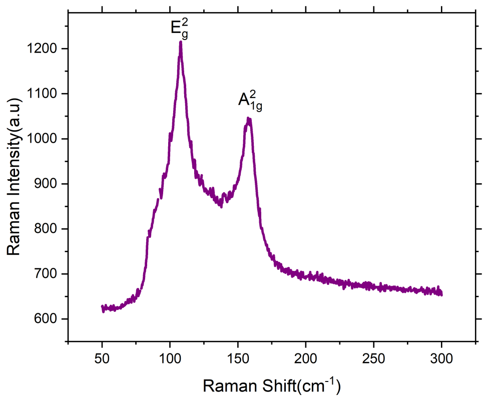


(b) Raman shift for IBST sample.

FIG. 5: Raman spectra of BST and IBST films.

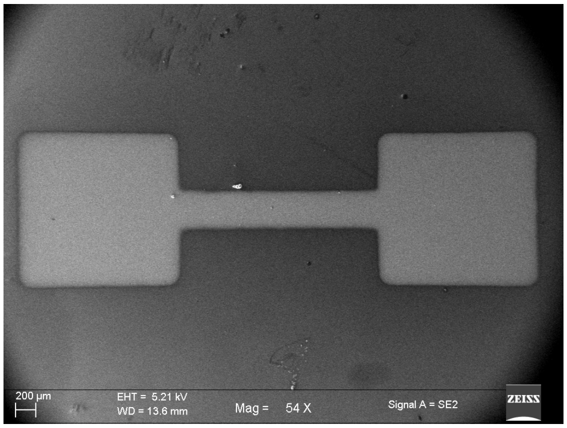


(a) Geometrical shape of our sample without contact pads.

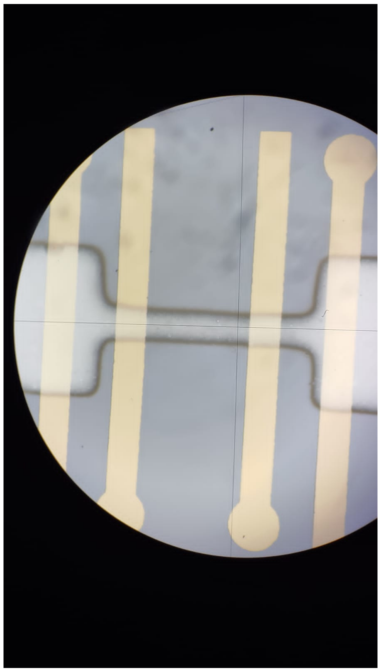

(b) Geometrical shape of our sample with contact pads.

FIG. 6: Shows the dumbell shape of our sample.

**VIII. Experimental Setup and Digital Signal Processing:**

In our experimental setup, shown in Fig. 7, we have utilised a lock-in amplifier (LIA) SR830 as a signal source and detector, which is commonly used in the low-frequency noise spectroscopy

experiments[3]. The reference frequency in our experimental setup was kept fixed at a value of 220 Hz. To convert a voltage source to a stable constant current source, we introduced a large series resistance to the sample. A constant current was subsequently directed through our sample using a four-probe technique, which is chosen for its ability to mitigate the impact of contact resistance and provide accurate measurements of intrinsic sample properties. The lock-in amplifier, configured with a 10 msec time constant, optimized the balance between noise suppression and signal response time. The processed output of channel 1 from the lock-in amplifier was fed into an NI-MyDAQ analog to digital converter with a sampling rate set to 16,384 samples per second. Analog signals were smoothly converted to digital format and stored on the computer for detailed analysis in later stages. Background noise was observable on Channel 1 when minimal constant current was applied to the sample, corresponding to the lock-in amplifier's minimum voltage of 4 mV, or on Channel 2, which provided an out-of-phase (background) signal.

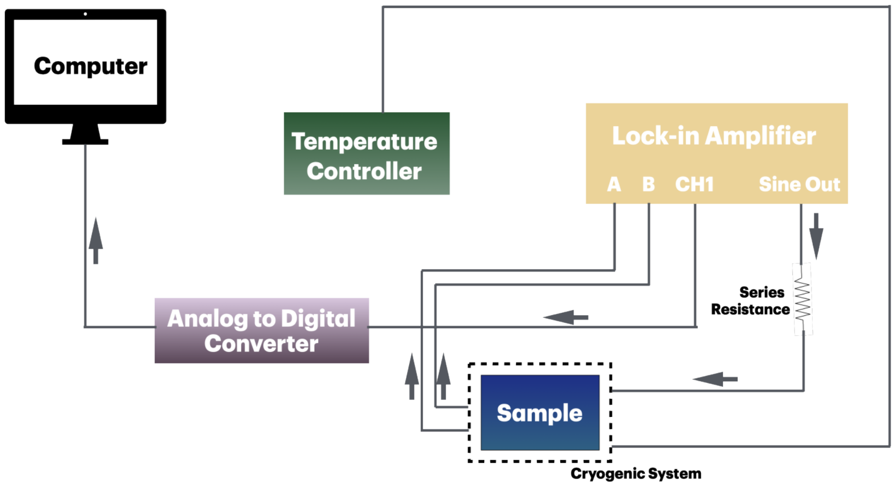


FIG. 7: Schematic of the experimental setup for noise measurements from room temperature down to 90 kelvin.

After acquiring the digitised data on the computer, we employed digital signal processing techniques, specifically the decimation technique[3]. Decimation involves a two-step process: low-pass filtering (LPF) followed by downsampling. The LPF serves to eliminate higher frequencies, ensuring that downsampling avoids aliasing effects. Aliasing is evident in Fig. 8, where a 4 Hz sinusoidal signal, sampled at 4 Hz, misleadingly appears as a 1 Hz signal due to aliasing. However, when the sampling rate exceeds twice the signal's frequency, the resulting sampled signal

faithfully represents the original. To optimise computer speed, we implemented a three-step decimation with downsampling factors of 16, 8, and 4, resulting in a final sampling rate of 32 Hz. According to Nyquist theorem, one can capture frequency components up to 16 Hz. Since the time constant was 10 ms, the signal was acquired till 10 Hz to stay away from the filter artefacts of the LPF of LIA.

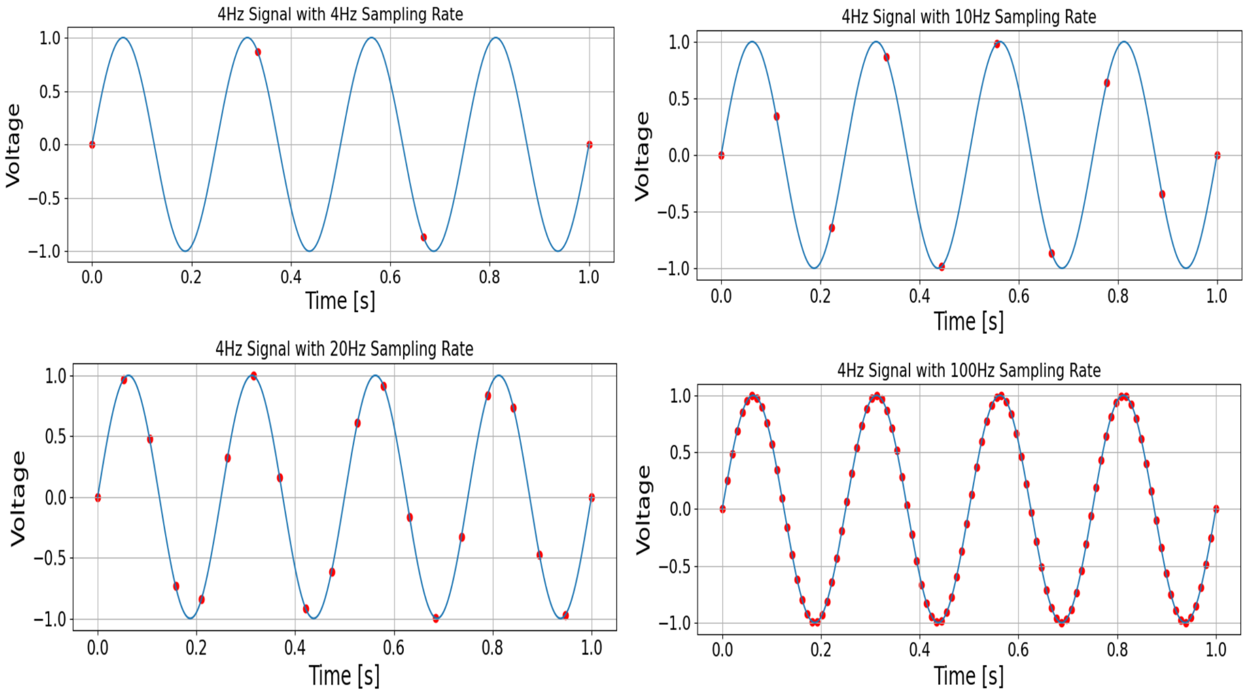


FIG. 8: When a 4 Hz sinusoidal signal (blue line) is sampled (red solid circles) at a rate of 4 Hz, it appears as a 1 Hz signal due to aliasing. However, if the sampling rate surpasses twice the signal's frequency—such as 10 Hz, 20 Hz, or 100 Hz—the sampled signal precisely retains the characteristics of the original.

We utilised the Kaiser window method, specifying the cutoff value and transition range, for the low-pass filtering. This method contributes to achieving a more refined and controlled filtering process. The final step involved obtaining the Power Spectral Density (PSD) using the Welch averaging method. We defined an ensemble number of 30 and applied a Hanning window during this process. Our focus was narrowed to a specific region of interest, spanning from 0.1 Hz to 10 Hz. This stringent selection allowed us to extract relevant frequency information within our specified range. The normalised estimation of the power spectral density obtained through the method described earlier has been verified by comparing it with the estimation of the same quantity using a commercially available Fast Fourier Transform program shown in Fig. 9. The PSD using

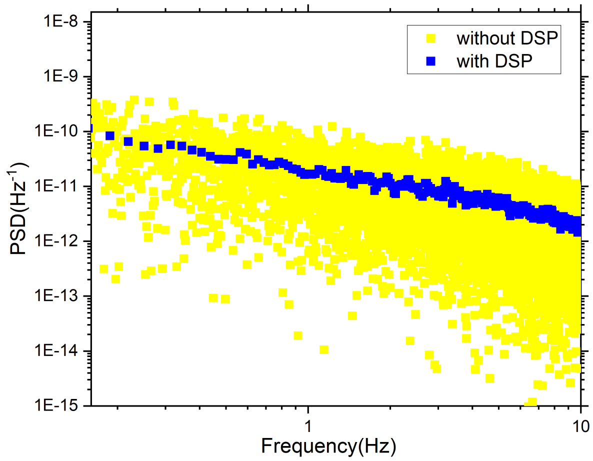


FIG. 9: Shows the normalized PSD with frequency of the raw data without DSP technique(yellow) using commercially available software and after DSP technique(blue).

commercial software shown in yellow, without decimation matches well with the blue data which was obtained after the decimation technique. The comparison of the quadrature component (red) of the noise versus the in-phase signal (pink) is shown in Fig. 10 for 100 Kohm samples.

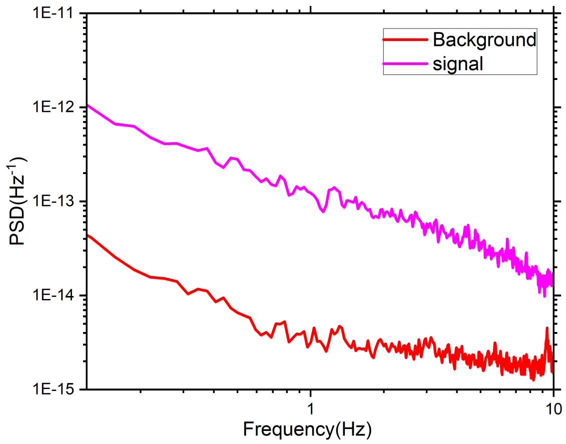


FIG. 10: Shows the signal(pink) is much higher than the out of phase signal(red).

## IX. Silicon wafer:

BST and IBST samples were deposited on a silicon wafer substrate, which underwent characterization through Raman spectroscopy. Raman spectra indicated the crystalline nature of the substrate, as depicted in Fig. 11[4].

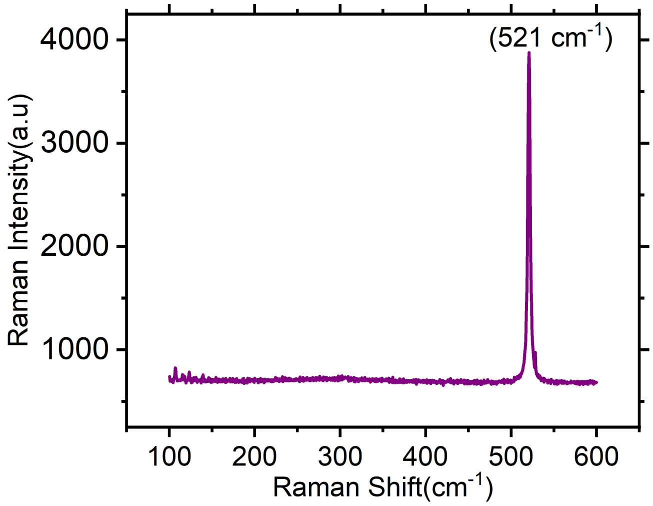


FIG. 11: Shows raman peak at $521cm^{-1}$.


[1] A. Pandey, S. Singh, B. Ghosh, S. Manna, R. Gopal, and C. Mitra, "Pulsed laser deposition of highly c-axis oriented thin films of bsts topological insulator," (2019), arXiv:1910.08100 [cond-mat.mtrl-sci].

[2] S. Singh, R. Gopal, J. Sarkar, A. Pandey, B. G. Patel, and C. Mitra, Journal of Physics: Condensed Matter **29**, 505601 (2017).

[3] A. Ghosh, S. Kar, A. Bid, and A. K. Raychaudhuri, "A set-up for measurement of low frequency conductance fluctuation (noise) using digital signal processing techniques," (2004), arXiv:cond-mat/0402130 [cond-mat.other].

[4] T. Deschaines, J. Hodkiewicz, and P. Henson, (2009).
